# Supplementary material for: Semi-Supervised 3D Hand Shape and Pose Estimation with Label Propagation
Source: arXiv:2111.15199 source file (2021-11-30)

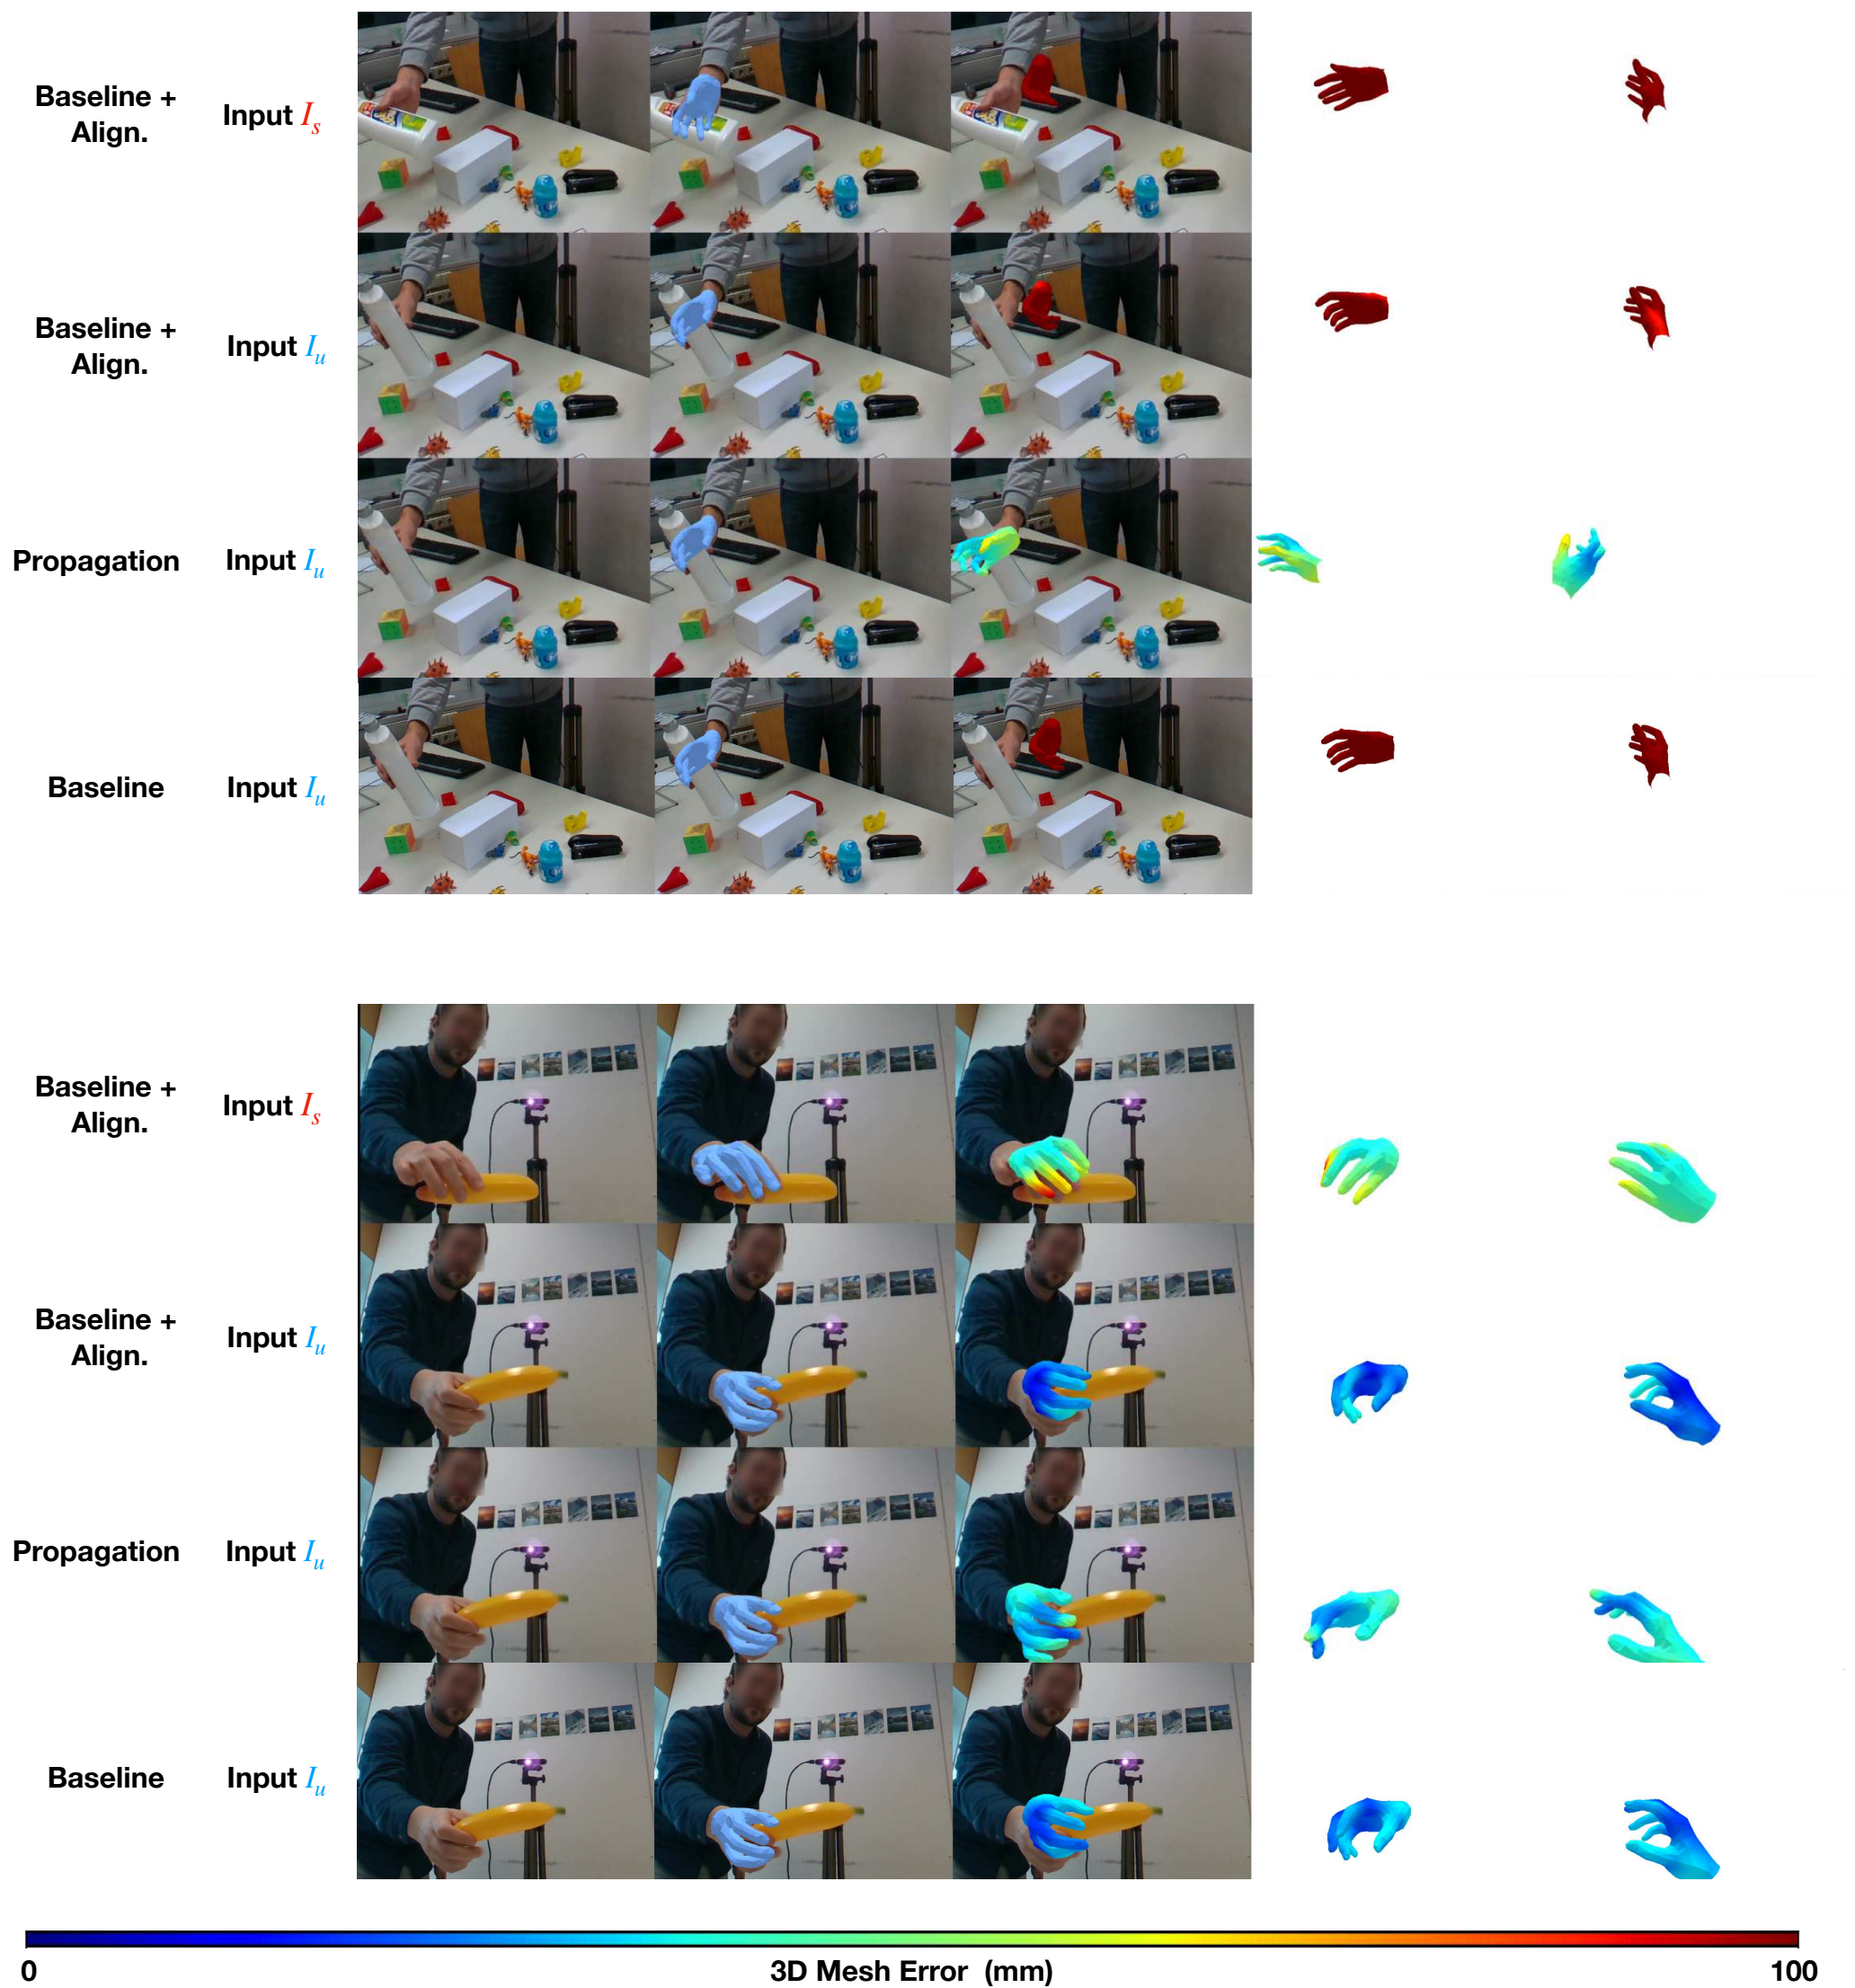



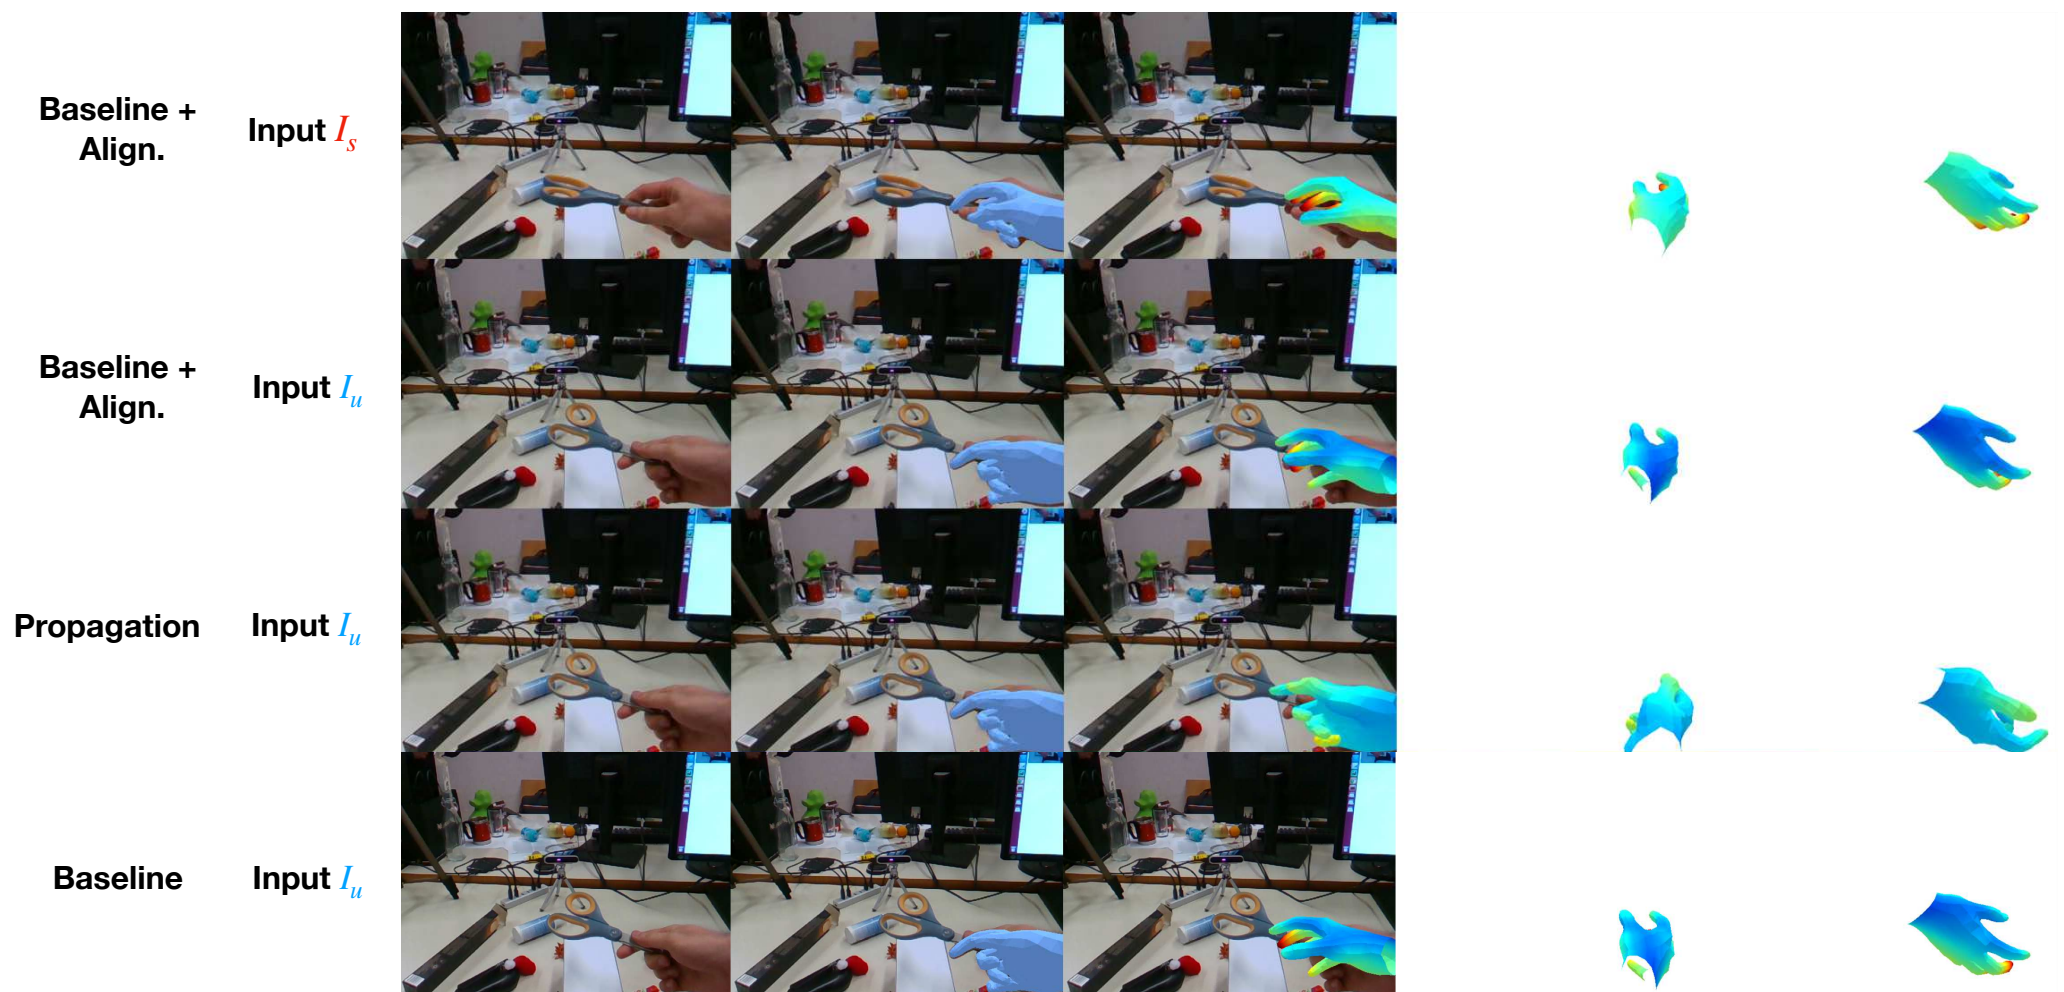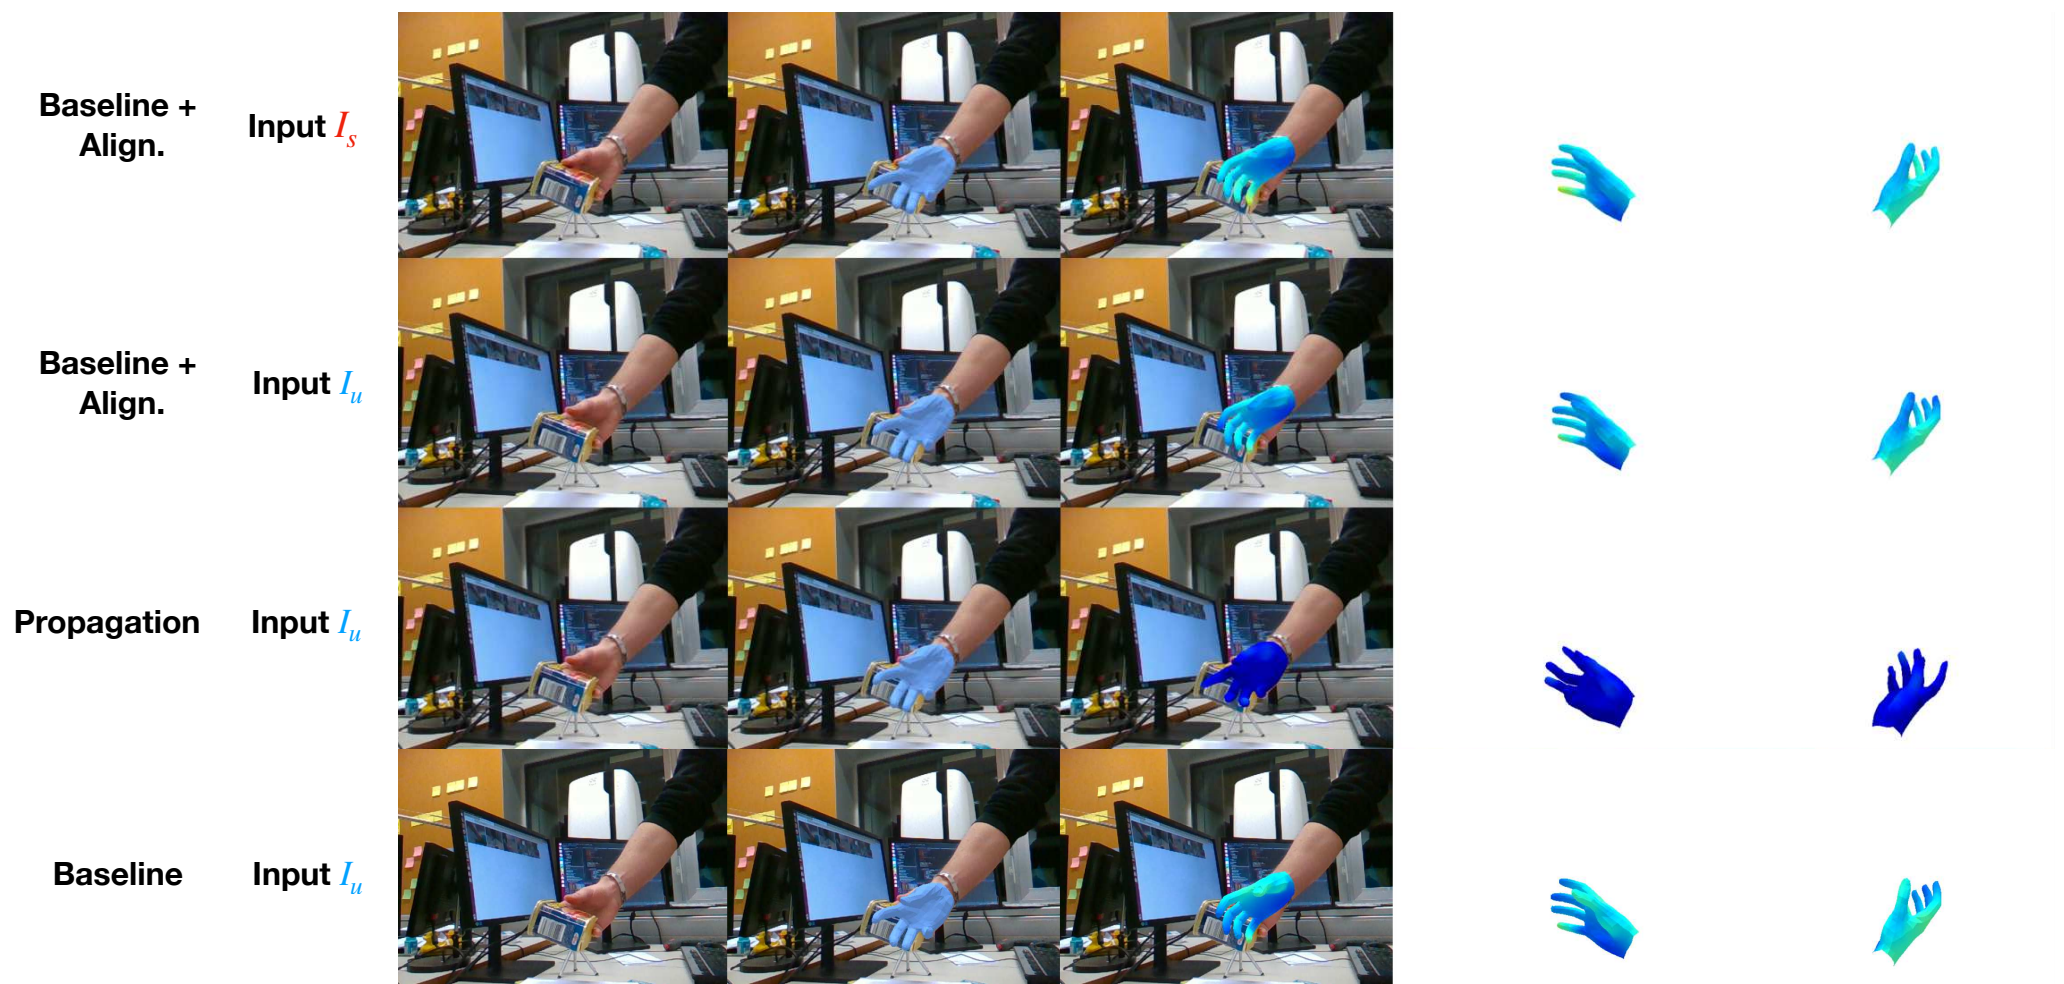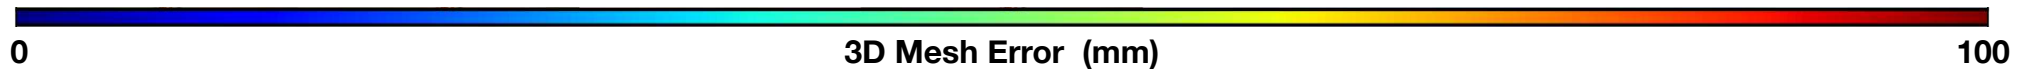

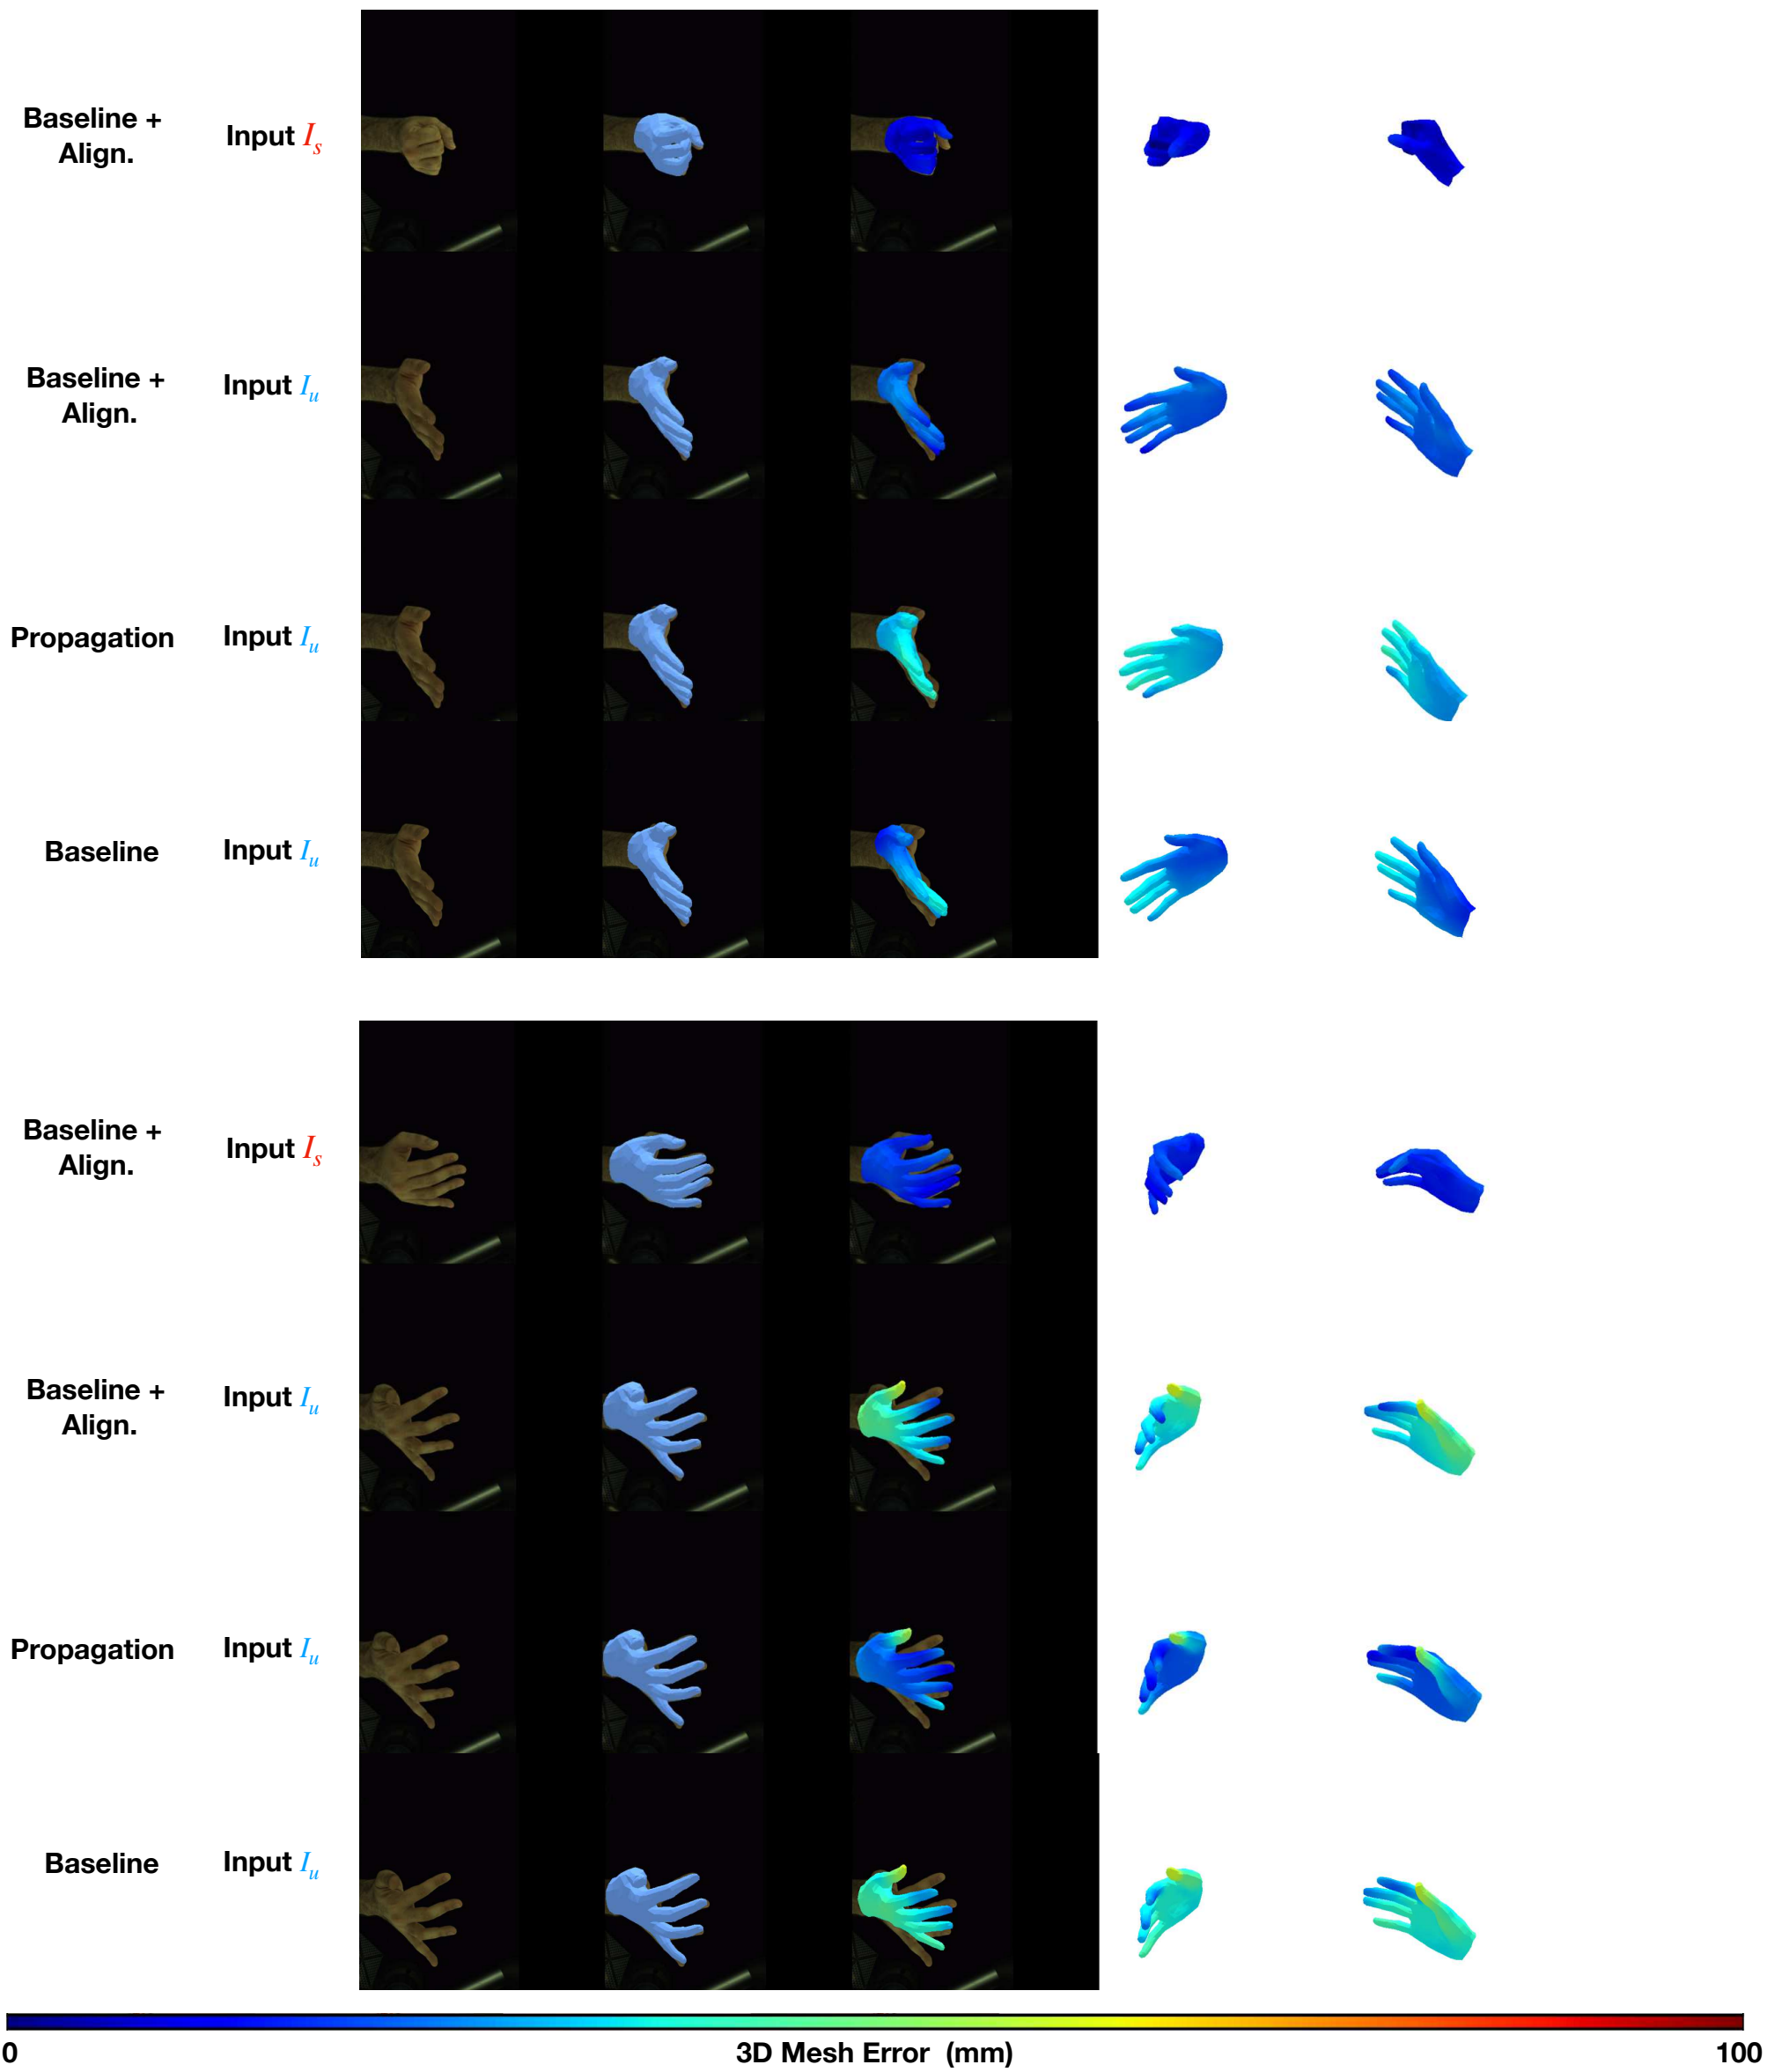



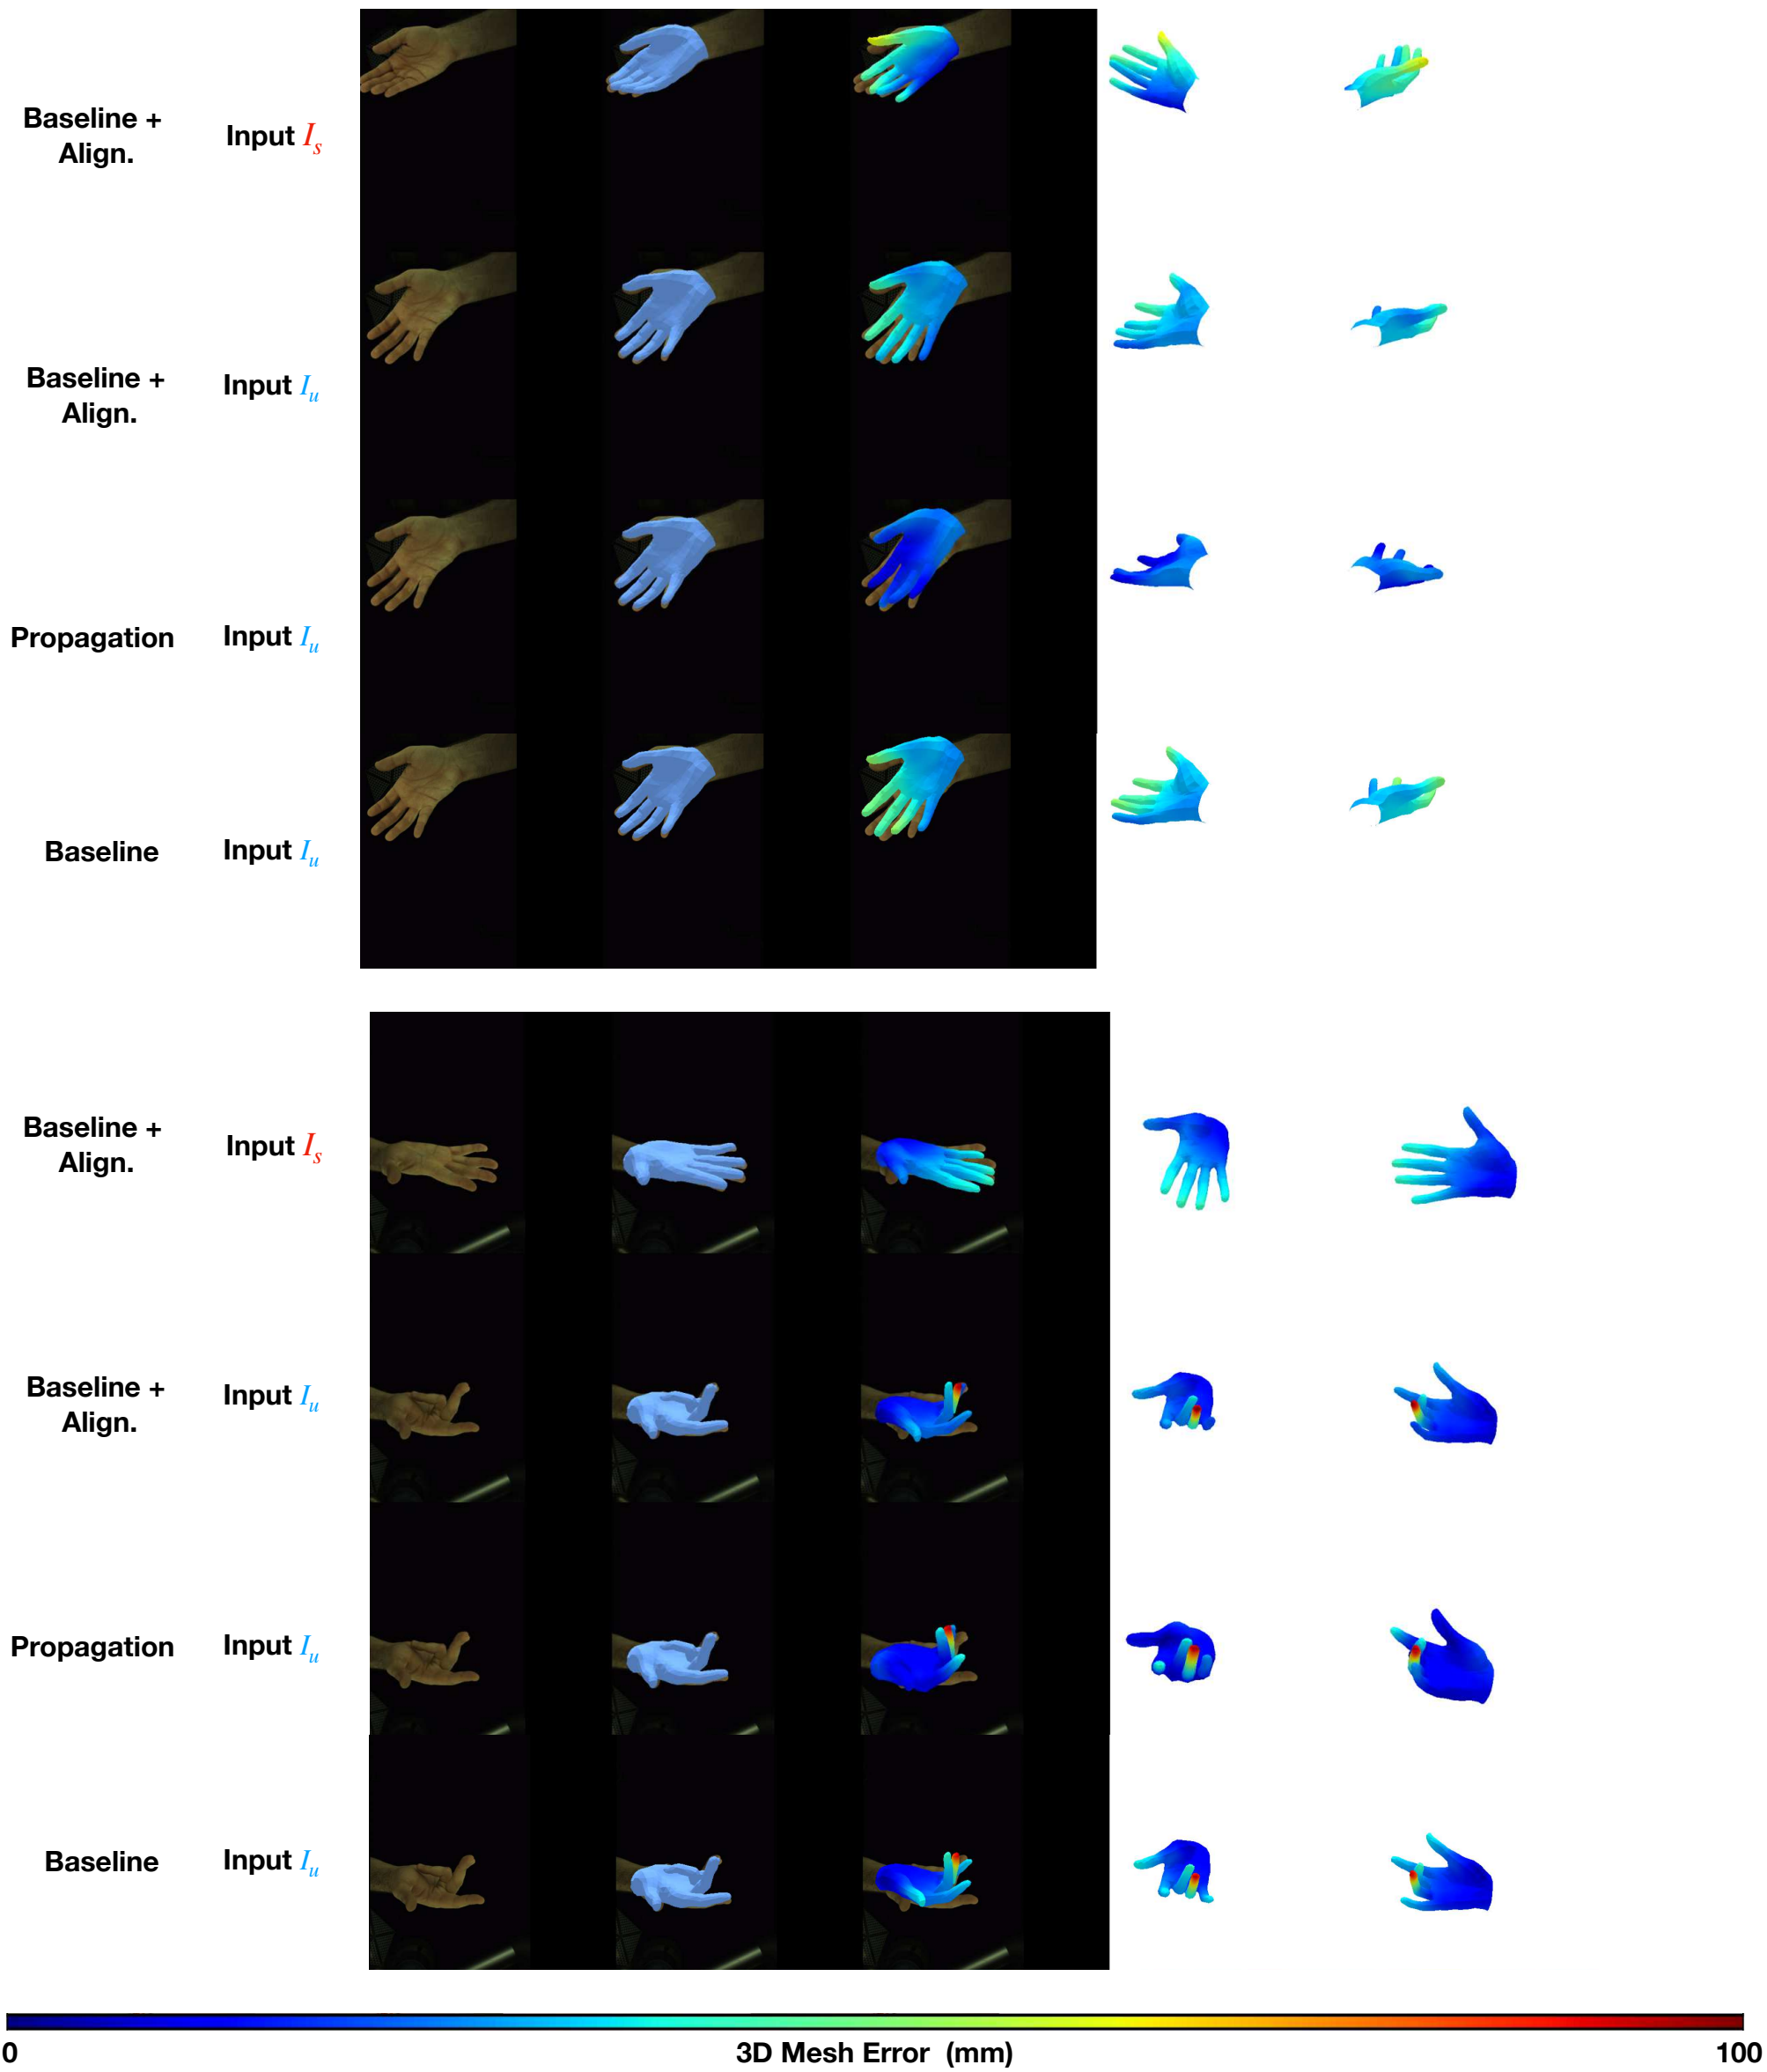

Supplement: Supplementary file 1 [file appendix.pdf]
